# Supplementary material for: Patchy Kinetic Sunyaev-Zel'dovich Effect with Controlled Reionization History and Morphology
Source: arXiv:2203.04337 source file (2022-03-08)
Supplement: Supplementary file 1 [file appendix.tex]

\appendix
\counterwithin{figure}{section}
\section{Visualization of Patchy kSZ Maps for Other Reionization Parameters}
\begin{figure*}[t]
\centering
\includegraphics[width=0.85\textwidth]{Appendix/maps_z50.pdf}
\includegraphics[width=0.85\textwidth]{Appendix/maps_az.pdf}
\includegraphics[width=0.85\textwidth]{Appendix/maps_mmin.pdf}
\includegraphics[width=0.85\textwidth]{Appendix/maps_mfp.pdf}
\caption{$10\times 10$ ${\rm degree}^2$ maps of the kSZ temperature fluctuation. A shorter reionization scenario ($\Delta_z=2$) results in a smoother kSZ map, because there is less small-scale electron number density fluctuation from high redshifts. A lengthened reionization ($\Delta_z = 6$) corresponds to more fluctuations on all scales because of the stacked ionized bubbles of different sizes along the line of sight.}
\label{fig:other_maps}
\end{figure*}
